# Supplementary material for: FwdLLM: Efficient FedLLM using Forward Gradient
Source: arXiv:2308.13894 source file (2024-01-20)
Supplement: Supplementary file 1 [file sec-appendix.tex]

\section*{Appendix} \label{sec:appendix}

\input{sec-appendix-models.tex}
